# Supplementary material for: Signature Cocycles on the Mapping Class Group and Symplectic Groups
Source: arXiv:1811.09357 source file (2020-04-13)
Supplement: Supplementary file 1 [file paper3-appendix1.tex]

%PAPER3-APPENDIX1.TEX (12.9.2018)
%OWNER Caterina

\appendix
\section{Homology and cohomology of groups}\label{app: hom and cohom}

Let $G$ be a discrete group, and $A$ a $\bZ[G]$-module.

The homology $H_n(G;A)$ and cohomology groups $H^n(G;A)$ ($n \geqslant 0$) are the abelian groups defined in terms of homological algebra by
$$\begin{array}{l}
H_n(G;A)~=~\Tor_n^{\bZ[G]}(\bZ,A)~=~H_n(P \otimes_{\bZ[G]}
 A)~,\\[1ex]
 H^n(G;A)~=~\Ext^n_{\bZ[G]}(\bZ,A)~=~H_n(\Hom_{\bZ[G]}(P,A))
  \end{array}
 $$
with $P$ a projective $\bZ[G]$-module resolution of $\bZ$ with the trivial $\bZ[G]$-action. In terms of the classifying space $BG$
$$H_n(G;A)~=~H_n(BG;A)~,~H^n(G;A)~=~H^n(BG;A)~(n \geqslant 0)~.$$
We shall only be concerned with the case when $A$ is an abelian group with the trivial $\bZ[G]$-action. The homology and cohomology groups are related by
the universal coefficient theorem exact sequence
$$0 \longrightarrow \Ext^1_{\bZ}(H_{n-1}(G;\bZ),A) \longrightarrow H^n(G;A) \longrightarrow \Hom_\bZ(H_n(G;\bZ),A) \longrightarrow 0~.$$
For $A=\bZ$ write
$$H_n(G;\bZ)~=~H_n(G)~,~H^n(G;\bZ)~=~H^n(G)$$
as usual. We shall only be concerned with the cases $n=1,2$, when the homology and cohomology groups have more direct expressions in terms of group theory.

\begin{defn}
Let $G$ be a group. \\
(i) The \emph{commutator}\index{commutator, $[x,y]$} of $x,y \in G$ is the element
$$[x,y]~=~xyx^{-1}y^{-1} \in G~.$$
For any subsets $X,Y \subseteq G$ let $[X,Y] \triangleleft G$ be the normal subgroup generated by the commutators $[x,y] \in G$ ($x \in X$, $y \in Y$).\\
(ii) The  \emph{first homology group}\index{homology group, first, $H_1(G)$} of $G$ is the abelian group
$$H_1(G)~=~G^{ab}~=~G/[G,G]~.$$
The group $G$ is {\it perfect} if $H_1(G)=0$, or equivalently $G=[G,G]$.\\
(iii) The  \emph{first cohomology group}\index{cohomology group, first, $H^1(G)$} of $G$ is the abelian group
$$H^1(G)~=~\Hom_{\bZ}(H_1(G),\bZ)~.$$
(iv) For any abelian group $A$,
$$H_1(G;A)~=~H_1(G)\otimes A~,~ H^1(G;A)~=~\Hom_\bZ(H_1(G),A)~.$$
\end{defn}

For any space $X$ and any abelian group $A$ there are defined isomorphisms
$$\begin{array}{l}
H^1(X;A) \longrightarrow \Hom_{\bZ}(H_1(X),A)~;~f \longmapsto (x \longmapsto f(x))~,
\\[1ex]
[X,BA] \longrightarrow H^1(X;A)~;~(f\colon X \longrightarrow BA) \longmapsto (f_*\colon\pi_1(X) \longrightarrow A)~.
\end{array}$$
It follows that for the classifying space $X=BG$ of a discrete group $G$ 
the function
$$H^1(G;A) \longrightarrow H^1(BG;A)~=~[BG,BA]~;~f \longmapsto Bf$$
is an isomorphism.

\begin{defn}\label{def: extension cocycle} Let $G$ be a group, and $A$ an abelian group.\\
{\rm (i)} A \emph{cocycle}\index{cocycle} is a function $\tau\colon G \times G \to A$ such that
$$\tau(x,y)+\tau(xy,z)=\tau(y,z)+\tau(x,yz) \in A~(x,y,z \in G)~.$$
{\rm (ii)} A cocycle $\tau$ determines a central extension 
$$1 \longrightarrow A \longrightarrow A\times_{\tau}G \longrightarrow G \longrightarrow 1$$
with the group structure on $A\times_{\tau}G=A \times G$ given by
$$(A\times_{\tau}G) \times (A\times_{\tau}G) \longrightarrow A\times_{\tau}G;((a,x),(b,y)) \longmapsto (a+b+\tau(x,y),xy)~.$$
{\rm (iii)} A \emph{cochain}\index{cochain} is a function $f\colon G \to A$, with
\emph{coboundary}\index{coboundary} the cocycle
$$\delta f\colon G \times G \longrightarrow A;(x,y) \longmapsto \delta f(x,y)=
f(x)+f(y)-f(xy)~.$$
{\rm (iv)} The \emph{second cohomology group}\index{cohomology group, second, $H^2(G,A)$} $H^2(G,A)$ is the abelian group of
equivalence classes $[\tau]$ of cocycles $\tau\colon G \times G \longrightarrow A$
with
$$\tau \sim \tau'~{\rm if}~\tau-\tau'=\delta f~\hbox{for some cochain
$f\colon G \to A$}~.$$
The addition is by the addition of cocycles.
\end{defn}

\begin{defn} (i) An \emph{extension}\index{extension} of 
a group $G$ by a group $R$ is  an exact sequence
$$1 \longrightarrow R \longrightarrow F \longrightarrow G \longrightarrow 1~,$$
so that $R$ is a normal subgroup of $F$.  \\
(ii) A \emph{presentation}\index{presentation} of a group $G$
is an extension $1\to R \to F \to G \to 1$ with $F$ free.
\end{defn}

\begin{defn}\label{H2} (Schur \cite{Schur:1904a}, Hopf \cite{Hopf:1942a}) The  \emph{second homology group}\index{homology group, second, $H_2(G)$} of a group $G$ is the abelian group defined for any presentation 
$1 \to R \to F \to G \to 1$  to be 
$$H_2(G)~=~R \cap [F,F]/[R,F]$$
with  a central extension
$$1 \longrightarrow H_2(G) \longrightarrow [F,F]/[R,F] \longrightarrow [F,F]/R \cap [F,F] \longrightarrow 1~.$$
If $G$ is perfect then $[F,F]/R \cap [F,F] =G$.
\end{defn}

\begin{eg} The second homology group of a free group $F$ is
$H_2(F)=0$.
\end{eg}

\begin{defn} (i) An extension $1 \to A \to B \to G \to 1$
of a group $G$ is \emph{central}\index{central extension} if $A$ is in the centre of $B$ (i.e. $A$ is abelian and the action of $G$ on $A$ is trivial).\\
(ii) A {\it morphism}\index{central extension!morphism} of central
extensions
$$1 \longrightarrow A \longrightarrow B \longrightarrow G \longrightarrow 1~,~1 \longrightarrow A' \longrightarrow B' \longrightarrow G \longrightarrow 1$$ 
is a commutative diagram of exact sequences
$$\xymatrix{1 \ar[r] & A \ar[d]_-{f} \ar[r] & B \ar[d]_-{g} \ar[r] &
G \ar[r] \ar@{=}[d] & 1\phantom{.} \\
1 \ar[r] & A' \ar[r] & B' \ar[r] & G \ar[r] & 1.}$$ 
The morphism is an {\it isomorphism}\index{central extension!isomorphism}
if $f\colon A \to A'$ and $g\colon B \to B'$ are isomorphisms.\\
(iii) A central extension $1 \to A \to B \to G \to 1$ \emph{splits}\index{central extension!split} if there is an isomorphism
$$\xymatrix{1 \ar[r] & A \ar@{=}[d] \ar[r] & B \ar[d]_-{\cong} \ar[r] &
G \ar[r] \ar@{=}[d] & 1\phantom{,} \\
1 \ar[r] & A \ar[r] & A \times G \ar[r] & G \ar[r] & 1,}$$ 
i.e. if $B\to G$ is a split surjection.\\
(iv) The \emph{sum}\index{central extension!sum}  of central extensions
$$\begin{array}{l}
\xymatrix{1 \ar[r] & A \ar[r]^-{i_1} & B_1 \ar[r]^-{j_1} & G \ar[r] & 1,}\\
\xymatrix{1 \ar[r] & A \ar[r]^-{i_2} & B_2 \ar[r]^-{j_2} & G \ar[r] & 1\phantom{,}}
\end{array}$$
is the central extension 
$$\begin{array}{l}
\xymatrix{1 \ar[r] & A \ar[r]^-{i_{12}} & B_{12} \ar[r]^-{j_{12}} & G \ar[r] & 1}~,\\[1ex]
B_{12}~=~\dfrac{\{(x_1,x_2) \in B_1 \oplus B_2 \,\vert\,j_1(x_1)=j_2(x_2) \in G\}}{\{(i_1(a),i_2(a))\,\vert\,a \in A\}}~,\\[3ex]
i_{12} \colon A \longrightarrow B_{12}~;~a \longmapsto [(i_1(a),0)]=[(0,-i_2(a))]~,\\[1ex]
j_{12} \colon B_{12} \longrightarrow G~;~[x_1,x_2] \longmapsto j_1(x_1)=j_2(x_2)~.
\end{array}$$
\end{defn}

Central group extensions $1 \to A \to B \to G \to 1$ are classified by the second cohomology group $H^2(G;A)$, which is defined using cocycles, as follows.

\begin{prop} \label{le:commutator} Let
$$\xymatrix{1 \ar[r] & A \ar[r] & B \ar[r]^-{\displaystyle{p}} & G\ar[r] & 1}$$
be a central extension of a group $G$. \\
{\rm (i)} For any section $s\colon G \to B$ of $p$ the function
$$\tau_s\colon G \times G \longrightarrow A~;~(u,v) \longmapsto s(u)s(v)s(uv)^{-1}$$
is a cocycle such that the function
$$A \times_{\tau_s} G \longrightarrow B~;~(a,g) \longmapsto a s(g)=s(g)a$$
is an isomorphism with inverse
$$B \longrightarrow A \times_{\tau_s}G~;~x \longmapsto (x(sp(x))^{-1},p(x))~,$$
and defines an isomorphism of central extensions
$$\xymatrix{1 \ar[r] & A \ar@{=}[d] \ar[r] & A \times_{\tau_s} G \ar[d]_-{\displaystyle{\cong}} 
\ar[r] & G \ar@{=}[d] \ar[r] & 1\phantom{.}\\
1 \ar[r] & A  \ar[r] & B \ar[r] & G  \ar[r] & 1.}$$
{\rm (ii)}  The function
$$[s(~),s(~)]\colon G \times G \longrightarrow B~;~(u,v) \longmapsto [s(u),s(v)]$$
is independent of $s$, with $p([s(u),s(v)])=[u,v] \in G$.\\
{\rm (iii)} $H^2(G;A)$ is the abelian group of isomorphism classes of
central extensions $1 \to A \to B \to G \to 1$, with addition by the sum of
central extensions, and the isomorphism class of any split extension as zero.
\end{prop}
\begin{proof} (i) By construction.\\
(ii)  Every element of $A$ is central in $G$. If $s,s'$ are two sections of $p$ then the function
$$f\colon G \longrightarrow A=\mathsf{ker}\left(p\right)~;~u \longmapsto s'(u)s(u)^{-1}$$
is such that $s'(u)=f(u)s(u)=s(u)f(u) \in G$, so that for any $u,v \in G$
\begin{align*}
[s'(u),s'(v)]&= s(u)s(v)s(u)^{-1}s(v)^{-1}f(u)f(v)f(u)^{-1}f(v)^{-1}\\
&= s(u)s(v)s(u)^{-1}s(v)^{-1} = [s(u),s(v)] \in B.
\end{align*}
(iii) If $\tau,\tau'\colon G \times G \to A$ are cocycles such that
$\tau-\tau'=\delta f$ for a cochain $f\colon G \to A$ the function
$$g\colon A\times_{\tau}G \longrightarrow A\times_{\tau'}G~;~(a,x) \longmapsto (a+f(x),x)$$
defines an isomorphism of central extensions
$$\xymatrix{1 \ar[r] & A \ar@{=}[d] \ar[r] & A \times_{\tau} G \ar[d]^-{g}_-{\displaystyle{\cong}} 
\ar[r] & G \ar@{=}[d] \ar[r] & 1\phantom{.} \\
1 \ar[r] & A  \ar[r] & A\times_{\tau'}G \ar[r] & G  \ar[r] & 1.}$$

\vspace*{-1.3\baselineskip}
\end{proof}

For any group $G$ and abelian group $A$ the universal coefficient theorem 
gives a split exact sequence
$$0 \longrightarrow \Ext^1_{\bZ}(H_1(G),A) \longrightarrow H^2(G;A) \longrightarrow \Hom_\bZ(H_2(G),A) \longrightarrow 0~.$$

\label{UCA map}Let $G$ be a group defined by a presentation
\[
\xymatrix
{
1 \ar[r] & R \ar[r] &  F\ar[r]  & G=F/R \ar[r] & 1.
}
\]
Let 
\[
\xymatrix
{
1 \ar[r] & A \ar[r] &  \tilde{G}\ar[r]  & G \ar[r] & 1
}
\]
be a central extension of $G$ by the abelian group $A$. Consider
\[
\xymatrix
{
1 \ar[r] & R \ar[r]\ar[d]^\phi &  F\ar[r]\ar[d]^\phi  & F/R \ar[r]\ar[d]^= & 1\phantom{,}\\ 
1 \ar[r] & A \ar[r] &  \tilde{G}\ar[r]  & G \ar[r] & 1,
}
 \] where $\phi$ is chosen such as to produce a commutative diagram of extensions.
Note that $\phi$ restricts to a map $[F, F]\rightarrow [\tilde{G}, \tilde{G}]$. Moreover, as $\phi(R)\leq A\leq Z(\tilde{G})$, we see that $\phi([R, F])=\{1\}$. There is thus an induced map
$$
\begin{array}{lclc}
\bar{\phi}\colon &R\cap [F, F]/[R, F]&\longrightarrow& A\cap [\tilde{G}, \tilde{G}]\\\
	& r[R, F]&\longmapsto& \phi(r).
\end{array}$$
This is the map $H^2(G; A)\rightarrow \mathsf{Hom}_\bZ(H_2(G), A)$ from the universal coefficient theorem.

Suppose now that $\tilde{G}=F/[R, F]$, $A=R/[R, F]$ and $R\subset[F, F]$. Then $A=H_2(G)$ by Definition \ref{H2} and $\phi$ is the natural map $f\mapsto f[R, F]$. The induced map $\bar{\phi}$ is then the identity in $\mathsf{Hom}_\bZ(H_2(G), H_2(G))$.

\begin{propqed}
For a perfect group $G$ and any abelian group $A$ the universal coefficient
theorem gives a natural isomorphism 
$$H^2(G;A)~\cong~\Hom_{\bZ}(H_2(G),A)$$
sending the classifying element $(1 \to A \to B \to G \to 1) \in H^2(G;A)$
of a central extension to a $\bZ$-module morphism $H_2(G) \to A$ which fits into an exact sequence
\begin{equation*}
H_2(B) \longrightarrow H_2(G) \longrightarrow A \longrightarrow H_1(B) \longrightarrow H_1(G)=0~.
\qedhere
\end{equation*}
\end{propqed}

\begin{defn} A central extension $1 \to A \to B \to G \to 1$ is \emph{universal}\index{central extension!universal} if for every central extension $1 \to C \to D \to G \to 1$ there is a unique group morphism $B \to D$ such that the composite $B \to D \to G$ is the given map $B \to G$, i.e. there is a unique morphism of exact sequences
$$\xymatrix{
1 \ar[r] & A \ar[d] \ar[r] & B \ar[d] \ar[r] &
G \ar@{=}[d] \ar[r] &  1\phantom{.}\\
1 \ar[r] & C \ar[r] & D \ar[r] &G \ar[r] & 1.}$$
\end{defn}

\endinput

\begin{prop} \label{KM}
{\rm (Kervaire \cite{Kervaire:1970a}, Milnor \cite[Thms. 5.3,5.7, Cor. 5.8]{Milnor:1971a})}\\
{\rm (i)} A group $G$ has a universal central extension if and only if $G$ is
perfect, i.e. $H_1(G)=0$.\\
{\rm (ii)} A central extension $1 \to A \to B \to G \to 1$ of a perfect group $G$ is universal if and only if $B$ is perfect and the equivalent conditions hold :
\begin{itemize}
\item[(a)] $H_2(B)=0$,
\item[(b)] the universal coefficient theorem surjection sends
$(1\to A \to B \to G \to 1) \in H^2(G;A)$ to a $\bZ$-module isomorphism
${\rm Hom}_\bZ(H_2(G),A)$,
\item[(c)] for any morphism of central extensions
$$\xymatrix{
1 \ar[r] & C \ar[d] \ar[r] & D \ar[d] \ar[r] &
G \ar@{=}[d] \ar[r] &  1\\
1 \ar[r] & A \ar[r] & B \ar[r] &G \ar[r] & 1}$$
the central extension $1 \to C \to D \to G \to 1$ splits.
\end{itemize}
\hfill\qed
\end{prop}

\begin{eg}  {\rm (Milnor \cite[Thm. 5.10]{Milnor:1971a})}\\
Let $\St(R)$ be the Steinberg group of a ring $R$. The groups $E(R)=[GL(R),GL(R)]$ and $\St(R)$ are perfect, and
$$1 \to K_2(R)=H_2(E(R)) \to \St(R) \to E(R) \to 1$$
is a universal central extension.\\
\hfill\qed
\end{eg}

\begin{prop} {\rm (Barge and Lannes \cite[Prop. 5.4.2]{Barge/Lannes:2008a})}
\label{H2braid} Let $G$ be a group with an extension
$$\xymatrix{1 \ar[r] & R \ar[r] & F \ar[r] &G \ar[r]& 1~.}$$
{\rm (i)} There is defined an exact sequence of abelian groups
$$H_2(F) \to H_2(G) \to R/[R,F] \to H_1(F) \to H_1(G) \to 0$$
with an isomorphism
$$\coker(H_2(F) \to H_2(G))~\cong~ R \cap [F,F]/[R,F]~.$$
{\rm (ii)} The central extension
$$1\to R/[R,F] \to F/[R,F] \to G \to 1$$
fits ino a commutative braid of exact sequences of groups

$$\braid{[R,F]}{F}{G}{R}{F/[R,F]}{R/[R,F]}$$
The universal coefficient theorem surjection $H^2(G;R/[R,F]) \to
{\rm Hom}_{\bZ}(H_2(G),R/[R,F])$ sends the classifying element
$(1 \to R/[R,F] \to F/[R,F] \to G \to 1) \in H^2(G;R/[R,F])$ to the morphism
$H_2(G) \to R/[R,F]$ in {\rm (i)}.\\
{\rm (iii)} If $1\to R \to F \to G \to 1$ is a presentation of $G$ (i.e. if $F$ is free) and $R \subseteq [F,F]$ then 
$$H_2(F)~=~0~,~H_2(G)~=~R \cap [F,F] /[F,F]~=~R/[R,F]$$ 
so that the classifying element $(1 \to H_2(G) \to F/[R,F] \to G \to 1) \in H^2(G;H_2(G))$ is sent to $1 \in \Hom_{\bZ}(H_2(G),H_2(G))$. If in addition
$G$ and $F/[R,F]$ are perfect then
$$1 \to H_2(G) \to F/[R,F] \to G \to 1$$
is a universal central extension.\\
{\rm (iv)} The central extension
$$1 \to H_2(G) \to [F,F]/[R,F] \to [G,G] \to 1$$
fits into a commutative braid of exact sequence of groups

\bigskip

$$\xymatrix@H=15pt@!C=25pt{
0 \ar[dr] \ar@/^1.6pc/[rr] && R/[R,F]\ar[dr] \ar@/^1.6pc/[rr] && H_1(F)  \ar[dr] \ar@/^1.6pc/[rr] && 0\\
 & H_2(G)\ar[ur] \ar[dr] && F/[R,F] \ar[ur] \ar[dr] && 
 H_1(G) \ar[ur] \ar[dr] &\\ 
 H_2(F) \ar[ur] \ar@/_1.6pc/[rr] && [F,F]/[R,F] \ar[ur] \ar@/_1.6pc/[rr] && G 
  \ar[ur] \ar@/_1.6pc/[rr] && 0 }$$

    \bigskip  
    \bigskip
    
\noindent If $[G,G]$ and $[F,F]/[R,F]$ are perfect then $1 \to H_2(G)
\to [F,F]/[R,F] \to [G,G] \to 1$ is a universal central extension.\\
 \hfill\qed
\end{prop}

\begin{eg} (Barge and Lannes \cite[\S5]{Barge/Lannes:2008a}) Let $R$ be a commutative ring, with the identity involution. For any $g \geqslant 1$ let
$$H~:~\GL(g,R) \to \Sp(2g,R)~;~\alpha \mapsto \begin{pmatrix} \alpha & 0 \\
0 & (\alpha^*)^{-1} \end{pmatrix}$$
be the hyperbolic map, let $\Symm(g,R) \subset M_{g,g}(R)$ be the abelian group of symmetric $g \times g$ matrices over $R$, and define the group morphisms
$$\begin{array}{l}
E_0~:~\Symm(g,R) \to \Sp(2g,R)~;~\phi_0 \mapsto
\begin{pmatrix} 1 & 0 \\ \phi_0 & 1 \end{pmatrix}~,\\[2ex]
E_1~:~\Symm(g,R) \to \Sp(2g,R)~;~\phi_1 \mapsto
\begin{pmatrix} 1 & \phi_1 \\ 0 & 1 \end{pmatrix}~.
\end{array}$$
The general linear group $\GL(g,R)$ has two left actions on $\Symm(g,R)$ 
$$\begin{array}{l}
\GL(g,R) \times \Symm(g,R) \to \Symm(g,R)~;~ (\alpha,\phi_0) \mapsto
(\alpha^*)^{-1}\phi_0 \alpha^{-1}~,\\[2ex]
\GL(g,R) \times \Symm(g,R) \to \Symm(g,R)~;~ (\alpha,\phi_1) \mapsto
\alpha \phi_1 \alpha^*~.
\end{array}$$
Write the image of the induced group morphism 
$$\rho(g,R)~:~(E_0 * E_1)\rtimes H~:~
\widetilde{\widetilde{\Gamma}}(g,R)~=~
\Symm(g,R) * \Symm(g,R) \rtimes \GL(g,R) \to \Sp(2g,R)$$
as
$$\Gamma(g,R)~=~\mathsf{Im}\left(\rho(g,R)\right)~=~\ESp(2g,R) \cdot \GL(g,R) \subseteq \Sp(2g,R)~.$$
Apply Proposition \ref{H2braid} with
$$1 \to H~=~\mathsf{ker}\left(\rho(g,R)\right) \to F~=~\widetilde{\widetilde{\Gamma}}(g,R)
\to G~=~\Gamma(g,R) \to 1$$
and set
$$\widetilde{\Gamma}(g,R)~=~\widetilde{\widetilde{\Gamma}}(g,R)/
[\ker(\rho(g,R)),\widetilde{\widetilde{\Gamma}}(g,R)]$$
to obtain a central extension
$$1 \to A(R)=\Ker(\rho(g,R))/[\Ker(\rho(g,R)),\widetilde{\widetilde{\Gamma}}(g,R)]
\to \widetilde{\Gamma}(g,R) \to \Gamma(g,R) \to 1$$
which fits into a commutative braid of exact sequences
$$\xymatrix@R=15pt@C=-20pt{
 [H,F]=[\Ker(\rho(g,R)),\widetilde{\widetilde{\Gamma}}(g,R)] \ar[dr] \ar@/^1.6pc/[rr] && F=\widetilde{\widetilde{\Gamma}}(g,R)
 \ar[dr] \ar@/^1.6pc/[rr]^-{\rho(g,R)} &&  G=\Gamma(g,R) \\
  & H=\Ker(\rho(g,R))
  \ar[ur] \ar[dr] && F/[H,F]=\widetilde{\Gamma}(g,R)
  \ar[ur] \\ && H/[H,F]=A(R)
  \ar[ur]}$$

\hfill\qed
\end{eg}

\begin{prop}  Let $G$ be a group with an extension
$$\xymatrix{1 \ar[r] & R \ar[r] & F \ar[r] &G \ar[r]& 1}$$
with $F$ free.\\
{\rm (i)} {\rm (Eckmann, Hilton and Stammbach \cite[Thm. 2.1]{Eckmann/Hilton/Stammbach:1972a})} 
For a central extension 
$$1 \to A \to G \to Q \to 1$$
there is defined a commutative braid of exact sequences of groups

$$\braid{R}{F}{Q}{S}{G}{A}$$

\noindent  with 
$$S ~=~A \times_GF~=~\{(x,y) \in A \times F\,\vert\,[x]=[y] \in G\}~.$$
There is also defined a commutative braid of exact sequences of abelian groups

$$\xymatrix@R=15pt@!C=40pt{
R\cap [S,F]/[R,F] \ar[dr] \ar@/^1.6pc/[rr] && R/[R,F]\ar[dr] \ar@/^1.6pc/[rr] && H_1(F)  \ar[dr] \ar@/^1.6pc/[rr] && H_1(Q)\\
 & H_2(G)\ar[ur] \ar[dr] && S/[S,F] \ar[ur] \ar[dr] && 
 H_1(G) \ar[ur] \ar[dr] &\\ 
H_2(F)=0 \ar[ur] \ar@/_1.6pc/[rr] && H_2(Q)=S \cap [F,F]/[S,F] \ar[ur] \ar@/_1.6pc/[rr] && S/R[S,F]=A 
  \ar[ur] \ar@/_1.6pc/[rr] && 0 }$$

\bigskip

\noindent with an isomorphism
$$H^2(Q,A)~\cong~\coker(\Hom_{\bZ}(H_1(F),A)\to \Hom_{\bZ}(S/[S,F],A))$$
sending $(1\to A \to G \to Q \to 1) \in H^2(Q,A)$ to the morphism 
$S/[S,F] \to A$ induced by the surjection $S \to A$.
The surjection in the universal coefficient theorem split exact sequence
$$0 \to \Ext^1_{\bZ}(H_1(Q),A) \to H^2(Q,A) \to \Hom_{\bZ}(H_2(Q),A) \to 0$$
sends $(1\to A \to G \to Q \to 1)$ to the composite $H_2(Q) \to S/[S,F] \to A$.\\
{\rm (ii)} If $R\subseteq [F,F]$ (or equivalently $H_1(F) \cong H_1(G)$) then the central
extension
$$1 \to H_2(G)=R \cap [F,F]/[R,F]=R/[R,F]
\to \widetilde{G}=F/[R,F] \to G=F/R \to 1$$
is classified by 
$1 \in H^2(G;H_2(G))={\rm Hom}_\bZ(H_2(G),H_2(G))$.\\
{\rm (iii)} If $G$ is perfect  the universal coefficient theorem gives an isomorphism
$$H^2(G,A)~\cong~\Hom_{\bZ}(H_2(G),A)$$
sending a central extension $1 \to A \to E \to G \to 1$ to
an abelian group morphism $H_2(G) \to A$ which fits into a morphism of exact sequences
$$\xymatrix{
1 \ar[r] & H_2(G) \ar[d] \ar[r] & \widetilde{G} \ar[d] \ar[r] &
G \ar@{=}[d] \ar[r] &  1\\
1 \ar[r] & A \ar[r] & E \ar[r] &G \ar[r] & 1}$$
In particular, for $A=H_2(G)$ the element $1 \in H^2(G;H_2(G))={\rm Hom}_{\bZ}(H_2(G),H_2(G))$ classifies the central extension
$$1 \to H_2(G) \to \widetilde{G}=F/[R,F] \to G \to 0$$
given by {\rm (i)}.\\
\hfill\qed
\end{prop}

\section{Cohomology of Lie groups made discrete}

For any discrete group $G$ the group cohomology $H^2(G;\bZ)$ is isomorphic 
to the degree two cohomology $H^2(BG;\bZ)$ of the classifying space $BG$.
It classifies central group extensions\index{central extension}
\[ 1 \to \bZ \to \tilde G \to G \to 1. \]
For abelian $G$ a bilinear pairing $\tau\colon G \times G \to \bZ$ defines a cocycle 
classifying the central group extension
$$1 \to \bZ \to \bZ\times_{\tau} G \to G \to 1$$
with
$$\bZ \times_\tau G=\{(m,a)\,\vert\,m \in \bZ,a \in G\}~,~
(m,a)(n,b)=(m+n+\tau(a,b),a+b)~.$$

A (finite dimensional) Lie group $G$ has a classifying space\index{classifying space} 
$BG$ as a topological group. The singular cohomology $H^2(BG;\bZ)$ classifies 
covering groups\index{covering group}
\[ 1 \to \bZ \to \tilde G \to G \to 1 \]
where $\tilde G$ is again a Lie group.

We write $G^\delta$ 
for the same Lie group, but with the discrete topology.
Following Milnor \cite{Milnor:1983a} 
(see also Thurston \cite{Thurston:1974a}) we write $\bar G$ for
the homotopy fibre of $G^\delta \to G$. The goal of this section
is to recap some of what is known about the natural map 
$H^2(BG;\bZ)\to H^2(BG^\delta;\bZ)$.

\begin{eg}
Let $G=\bR$, the additive group of the real numbers. Since $G$ is 
contractible we have $\bar G = G^\delta$. \\
\indent Now $\bR$ is a $\bQ$-vector space of dimension equal to the 
cardinality of the continuum.
Since $\bQ$ is a filtered colimit of rank one free groups, 
we have $H_1(B\bQ^\delta)\cong \bQ$ and $H_i(B\bQ^\delta)=0$ 
for $i>1$. The K\"unneth theorem then gives 
$H_i(B\bR^\delta)\cong\Lambda^i_\bQ(\bR)$, the $i$th exterior
power of the reals over the rationals. This is a rational 
vector space of dimension equal to the continuum. 
By the universal coefficient theorem, 
\[ H^i(B\bR^\delta;\bZ) \cong \Ext(\Lambda^{i-1}_\bQ(\bR),\bZ), \] 
which is again a large rational vector space (note that $\Ext(\bQ,\bZ)$ 
is already an uncountable dimensional rational vector space).\\
\hfill\qed
\end{eg}

\begin{eg}
Let $G=U(1)\cong S^1$. The universal cover of $G$ is $\bR$, so
we have a pullback square
\[ \xymatrix{\bR^\delta \ar[r] \ar[d] & \bR \ar[d] \\
G^\delta \ar[r] & G.} \]
Since $\bR$ is contractible, this implies that $\bar G=\bR^\delta$.
Thinking of $U(1)$ as a $K(\bZ,1)$, we have a fibre sequence
\[ K(\bZ,1)\to K(\bR^\delta,1) \to K(G^\delta,1) \to K(\bZ,2). \]
From this, an easy computation shows that
$H^1(BG^\delta;\bZ) \cong \bR/\bZ$, and
\[ H^2(BG^\delta;\bZ)\cong H^2(BU(1);\bZ) \oplus H^2(B\bR^\delta;\bZ), \]
a direct sum of $\bZ$ and a large rational vector space.\\
\hfill\qed
\end{eg}

More generally, it is shown in Sah and Wagoner \cite{Sah/Wagoner:1977a}
(page 623) that if $G$ is a simply connected Lie group such that
the simply connected composition factors of $G$ are either $\bR$
or isomorphic to universal covering groups of Chevalley groups\index{Chevalley groups}  
over $\bR$ or $\bC$ then the integral homology $H_2(BG^\delta)$
is a $\bQ$-vector space of dimension equal to the continuum.

\begin{eg}
Let us examine the real Chevalley group $\Sp(2g,\bR)$. In this case, 
the universal cover is given by 
\[ 1 \to \bZ \to \widetilde{\Sp(2g,\bR)} \to \Sp(2g,\bR) \to 1. \]
Thus
\[ H^2(B\Sp(2g,\bR)^\delta;\bZ) \cong H^2(B\Sp(2g,\bR);\bZ) 
\oplus H^2(B\widetilde{\Sp(2g,\bR)^\delta};\bZ) \]
is a direct sum of $\bZ$ and a $\bQ$-vector space of dimension equal to
the continuum. \\
\hfill\qed
\end{eg}

In light of the size of $H^2(BG^\delta;\bZ)$, we clearly need to
restrict the kind of cocycles we should consider, in order to identify
the central extensions which are also covering groups; namely those
that are in the image of $H^2(BG;\bZ)\to H^2(BG^\delta;\bZ)$.
It's clearly no use trying to restrict to continuous cocycles; for example
if $G$ is connected then the only continuous cocycles are the constant ones.
So what should we try?
This problem was solved by Mackey \cite{Mackey:1957a}, as follows.

Recall that given a topological space, the Borel sets\index{Borel set} are the smallest
collection of subsets containing the open sets, and closed under
complementation and arbitrary unions. A map is a Borel map if the
inverse image of every Borel set is a Borel set.
Theorem~7.1 of Mackey's paper
implies that under reasonably general conditions, if we're just given
the Borel sets and a group structure on $G$ consisting of Borel maps, then
there is a unique structure of locally compact topological group on $G$
for which these are the Borel sets and group structure. The proof
depends on Weil's converse to Haar's theorem on measures, 
described in Appendix 1 of Weil \cite{Weil:1940a}. In particular, the
topology can be obtained by taking for the neighbourhood system of the identity
element in $G$ the family of all sets of the form $A^{-1}A$, where $A$ is a Borel
set of positive measure.

The consequence of Mackey's theorem which we wish to describe is as follows.
Given a cocycle $G\times G \to \bZ$ which is also a Borel map then
consider the covering group
\[ 1 \to \bZ \to \tilde G \to G \to 1. \] 
The group $\tilde G$ inherits a Borel structure, as the underlying set is $G \times \bZ$.
This is compatible with the group structure, and so by Mackey's theorem
$\tilde G$ is a topological group in a unique way. Uniqueness of the
structure of topological group on $G$ implies that the topological group $\tilde G/\bZ$ is
isomorphic to $G$, and therefore the map $\tilde G \to G$ is continuous. 
It follows that $\tilde G$ is a Lie group.

So we define the Borel cohomology $H^2_b(G,\bZ)$ to be Borel cocycles
modulo coboundaries of Borel cochains $G \to \bZ$.

\begin{theorem}\label{th:Borel}
If $G$ is a Lie group then the image of the injective map $H^2(BG;\bZ)\to H^2(BG^\delta;\bZ)$ is
equal to the image of $H^2_b(G,\bZ) \to H^2(G^\delta,\bZ)$:
\[ \xymatrix{H^2(BG;\bZ) \ar[r] \ar[d]^\cong & H^2(BG^\delta;\bZ) \ar[d]^\cong \\
H^2_b(G,\bZ) \ar[r] & H^2(G^\delta,\bZ).} \]
\hfill\qed
\end{theorem}

\section{Cocycles on $S^{1\delta}$}

We are concerned in this section with certain Borel cocycles $\tau\colon S^{1\delta}\times S^{1\delta} \to \bZ$
on the (discrete) circle group ${S^{1\delta}}$, and the covering groups they define. We shall think  of $S^{1\delta}$ as the unit interval $[0,1]$ with the
endpoints identified, using the group isomorphism
$$[0,1]/(0 \sim 1)\xymatrix{\ar[r]^-{\cong}&} S^{1\delta}~;~a \mapsto e^{2\pi ia}$$
as an identification. 

The ``standard cocycle''\index{standard cocycle} is given by
$$ \tau ~:~[0,1) \times [0,1) \to \bZ~;~(a,b) \mapsto  \tau(a,b) = \begin{cases} 0 & \text{if } 0 \leqslant a+b < 1 \\ 1 & \text{if } 1 \leqslant a+b < 2. \end{cases}  $$
This defines the extension
\[ 1 \to \bZ \to \bR \to S^{1\delta} \to 1. \]
We shall say that a cochain $f$ is ``nice'' if it is piecewise constant. In other words, 
$S^1$ is divided into a finite number of intervals with open or closed ends, on 
each of which $f$ is constant. We shall say that a coboundary $\tau$ is ``nice"
if it is the coboundary of a nice cochain, and we shall say that a cocycle is
``nice''\index{nice cocycle} if it is the sum of a nice 
coboundary and an integer multiple $m$ times
the standard cocycle. Every nice cocycle defines a topological covering 
group of $S^1$, and by Theorem \ref{th:Borel} the quotient of the nice cocycles by the
nice coboundaries gives $H^2_b(S^1,\bZ) \cong \bZ$, with generator the class $[\tau]$ of the standard cocycle. 
The integer $m$, which we call the call the ``covering number''\index{covering number} of the cocycle $\tau$, is well defined. If $m=0$ then the
covering is trivial:
\[ 1 \to \bZ \to S^1 \times \bZ \to S^1 \to 1, \]
while if $m\ne 0$, the covering takes the form
\[ 1 \to \bZ \to \bR \times \bbZ{|m|} \to S^1 \to 1. \]

We can draw a picture of a nice cocycle $\tau$ in an obvious way, by dividing 
$[0,1]\times [0,1]$ into subregions where $\tau$ is constant.

For example, the
standard cocycle gives the following picture.
{\small
\begin{center}
\begin{picture}(80,80)
\put(10,10){\line(1,0){60}}
\put(10,70){\line(1,0){60}}
\put(10,10){\line(0,1){60}}
\put(70,10){\line(0,1){60}}
\put(10,70){\line(1,-1){60}}
\put(25,25){$0$}
\put(50,50){$1$}
\end{picture}
\end{center}
}%end small

\begin{theorem}\label{th:S1cocycle}
The picture of a nice cocycle has only horizontal, vertical and leading diagonal boundary lines.
The covering number can be computed by looking at the diagonal lines only. For each diagonal
line segment, we compute ((value of cocycle above the line segment) minus (value of cocycle
below the line segment)) $\times$ length of line segment, normalised so that the number of segments in the
main diagonal is equal to one. Adding these quantities gives the covering number.
\end{theorem}
\begin{proof}
The quantity described in the theorem is additive on nice cocycles, so we
only need check the theorem on the standard cocycle and on coboundaries.
For the standard cocycle, there is just one diagonal line segment, and the difference
in the values from below to above the line segment is one, so the theorem is true in
this case. For a nice coboundary $\delta f$, the diagonal lines happen where $f(a+b)$ 
changes in value. For each point in the unit interval where $f$ changes value, the
total normalised length of the one or two diagonal line segments representing the change
in value of $f(a+b)$ is equal to one. So we are adding the changes in value of $f$ as
$f$ goes once round $S^1$. The total is therefore zero.
\end{proof}

Notice that in this theorem, the values of $\tau$ on the boundaries of regions
is irrelevant to the computation of the covering number.

\begin{eg}\label{eg:two}
For any $p,q \in \bZ$ define the nice cochain
$$f(p,q)~:~[0,1) \to \bZ~;~a \mapsto \begin{cases} p&{\rm if}~0 \leqslant a < 1/2\\
 q&{\rm if}~1/2 \leqslant a <1
 \end{cases}$$
 with nice coboundary
 $$ \delta f(p,q)~:~[0,1) \times [0,1) \to \bZ~;~
 (a,b) \mapsto  f(a)+f(b)-f(a+b)~.$$
  For any $m \in \bZ$ the picture of the nice cocycle $m(\text{standard})+\delta f(p,q)$ has 8 regions
 $$\begin{tikzpicture}[scale=1.5]
\draw (0,0) -- (4,0) -- (4,4) -- (0,4) -- (0,0);
\draw (0,4) -- (4,0) ;
\draw (2,0) -- (2,4) ;
\draw (0,2) -- (4,2) ;
\draw (2,4) -- (4,2) ;
\draw (0,2) -- (2,0) ;
\draw (1,0.5) node{$p$} ;
\draw (1,1.5) node{$2p-q$};
\draw (1,2.5) node{$p$};
\draw (1,3.5) node{$m+q$};
\draw (3,0.5) node{$p$} ;
\draw (3,1.5) node{$m+q$};
\draw (2.7,2.5) node{$m-p+2q$};
\draw (3,3.5) node{$m+q$};
\end{tikzpicture}$$
with covering number
$${1 \over 2}((2p-q)-p)+(m+q-p)+{1 \over 2}((m+q)-(m-p+2q))~=~ m~.$$ 
\hfill\qed
\end{eg}

\begin{eg}\label{eg:MeyerS1}
We illustrate the theorem with the  two cases that will be of interest to us 
in understanding the Meyer cocycle $\tau_1$ of Definition \ref{df:Meyercocycle} for $g=1$
(Example \ref{eg:tau1})
$$\tau_1~:~[0,1] \times [0,1] \to \bZ~;~(a,b) \mapsto -2\sign(\sin(\pi a)\sin(\pi b)\sin(\pi(a+b)))~=~\begin{cases} -2&{\rm if}~
a+b<1\\
2&{\rm if}~a+b>1~.
\end{cases}$$
and the Maslov cocycle $\tau'_1$ of Definition \ref{df:Maslovcocycle} for $g=1$ (Example \ref{eg:tauprime1})
$$\tau'_1~:~[0,1] \times [0,1] \to \bZ~;~(a,b) \mapsto
-\sign(\sin(2\pi a)\sin(2\pi b)\sin(2\pi(a+b)))~.$$
The diagrams for these are as follows:

{\small
\begin{center}
\begin{picture}(80,80)
\put(10,10){\line(1,0){60}}
\put(10,70){\line(1,0){60}}
\put(10,10){\line(0,1){60}}
\put(70,10){\line(0,1){60}}
\put(10,70){\line(1,-1){60}}
\put(22,24){$-2$}
\put(50,50){$2$}
\end{picture}
\qquad\qquad
\begin{picture}(80,80)
\put(10,10){\line(1,0){60}}
\put(10,40){\line(1,0){60}}
\put(10,70){\line(1,0){60}}
\put(10,10){\line(0,1){60}}
\put(40,10){\line(0,1){60}}
\put(70,10){\line(0,1){60}}
\put(10,40){\line(1,-1){30}}
\put(10,70){\line(1,-1){60}}
\put(40,70){\line(1,-1){30}}
\put(13,14){$-1$}
\put(27.5,27.5){$1$}
\put(43,44){$-1$}
\put(57.5,57.5){$1$}
\put(43,14){$-1$}
\put(57.5,27.5){$1$}
\put(13,44){$-1$}
\put(27.5,57.5){$1$}
\end{picture}
\end{center}
}%end small

\noindent In the terminology of Example \ref{eg:two}
$$\begin{array}{l}
\tau_1~=~4({\rm standard})+\delta f(-2,-2)~,\\[1ex]
\tau'_1~=~4({\rm standard})+\delta f(-1,-3)
\end{array}$$
so that the covering number is equal to $4$ in both cases.  Now
$$f(1,-1)(a)~=~\sign (\sin 2 \pi a)~,$$
so that the cocycles differ by the coboundary
$$\begin{array}{ll}
\tau_1(a,b)-\tau'_1(a,b)&=~-\delta f(1,-1)(a,b)\\[1ex]
&=~-\sign(\sin 2\pi a)-\sign(\sin 2\pi b)+\sign(\sin 2\pi(a+b))~.
\end{array}$$
and
$$[\tau_1]~=~[\tau'_1]~=~4 \in H^2_b(S^{1 \delta},\bZ)~=~\bZ~.$$
\hfill\qed
\end{eg}

\section{Signature constructions of Wall, Maslov, and Meyer}\label{se:Meyer}

A lagrangian in a nonsingular symplectic form $(V,\fa)$ over $\bR$ with $V$ $2g$-dimensional is a linear subspace $L$ of dimension $g$
which is isotropic, meaning that for all $x,y\in L$ we have $\fa(x,y) = 0$.
If $L_1$, $L_2$ and $L_3$ are three lagrangians in $(V,\fa)$ we form the space
\[ \Delta= \Delta(L_1,L_2,L_3)= \{(a,b,c)\in L_1\oplus L_2 \oplus L_3 \mid a+b+c=0\in V\}. \]

\begin{lemma} \label{le:wall} 
{\rm (i)} The function
$$\fb\colon \Delta \times \Delta \to \bR; 
((a,b,c),(a',b',c')) \mapsto \fa(b,a') = -\fa(c,a') = \fa(c,b') $$
defines a symmetric form $(\Delta,\fb)$ over $\bR$. If the inclusions of the lagrangians are given by $j_i:(L_i,0) \to (V,\fa)$ $(i=1,2,3)$ then
$$(\Delta,\fb)~=~(\ker((j_1~j_2~j_3):L_1 \oplus L_2 \oplus L_3 \to V),
\begin{pmatrix} 0 & j_1^*\fa j_2 & 0 \\ 0 & 0 & 0 \\ 0 & 0 & 0 \end{pmatrix})~,$$
with radical
$$(\Delta,\fb)^{\perp}~=~\dfrac{(L_1 \cap L_2) \oplus (L_2 \cap L_3) \oplus (L_3 \cap L_1)}{L_1 \cap L_2 \cap L_3} \subseteq \Delta~.$$
{\rm (ii)} The symmetric form
$$(\Delta',\fb')~=~(\mathsf{ker}((j_3^*\fa j_1~j_3^*\fa j_2):L_1 \oplus L_2 \to L_3^*),\begin{pmatrix} 0 &j_1^* \fa j_2\\
0 & 0 \end{pmatrix})$$
is such that there is defined an isomorphism $f:(\Delta,\fb) \cong (\Delta',\fb')$ with
$$f~:~\Delta \to \Delta'~;~(a,b,c) \mapsto (a,b)~.$$
{\rm (iii)} If $j_3^*\fa j_2:L_2 \to L^*_3$ is an isomorphism there is defined
an isomorphism of symmetric forms
$$\begin{pmatrix}
1 \\ -(j_3^*\fa j_2)^{-1}(j_3^*\fa j_1)\end{pmatrix}~:~
(L_1,-(j_1^*\fa j_2)(j_3^*\fa j_2)^{-1}(j_3^*\fa j_1))
\xymatrix{\ar[r]^-{\cong}&} (\Delta',\fb')~.
$$
\end{lemma}
\begin{proof} (i) See Wall \cite{Wall:1969a}.\\
(ii)+(iii) Immediate from (i).
\end{proof}

\begin{rk} Let $\Sigma$ be a closed oriented surface, and let $M_1,M_2,M_3$ be oriented 3-dimensional manifolds with boundaries
$$\partial M_1~=~\partial M_2~=~\partial M_3~=~\Sigma~.$$
The thickening of $M_1 \cup_{\Sigma} M_2 \cup_{\Sigma} M_3$ is an oriented 4-dimensional manifold $N$ with boundary the disjoint union
$$\partial N~=~(M_1 \cup_{\Sigma} -M_2) \sqcup (M_2 \cup_{\Sigma} -M_3) \sqcup (M_3 \cup_{\Sigma} -M_1)~.$$
The nonsingular symplectic intersection form over $\bR$
$$(V,\fa)~=~(H_1(\Sigma;\bR),\phi_\Sigma)$$
has three lagrangians
$$L_i~=~\mathsf{ker}(H_1(\Sigma;\bR) \to H_1(M_i;\bR))~(i=1,2,3)$$
such that by \cite{Wall:1969a} the signature of $N$ is given by
$$\sigma(N)~=~-\sigma(\Delta(L_1,L_2,L_3),\fb) \in \bZ~.$$
\hfill\qed
\end{rk}

\begin{defn}
The \emph{Wall--Maslov index}\index{Wall-Maslov index} 
(Maslov \cite{Maslov:1965a}, Wall \cite{Wall:1969a}, Leray \cite{Leray:1981a}) 
of a triple of lagrangians $L_1,L_2,L_3$ in a nonsingular symplectic form
$(V,\fa)$ over $\bR$ is
$$\mu(L_1,L_2,L_3)~=~\sigma(\Delta,\fb)~=~
\sigma(\Delta',\fb') \in \bZ~.$$
\hfill\qed
\end{defn}

For any $g \geqslant 1$ the $2g$-dimensional real vector space $\bR^{2g}$ 
is  equipped with the standard nonsingular symplectic form 
$$ \begin{array}{l}
\langle~,~\rangle\colon \bR^{2g} \times \bR^{2g} \to  \bR; \\[1ex]
(x,y)=((x_1,x_2,\dots,x_{2g}),(y_1,y_2,\dots,y_{2g}))   \mapsto \langle x,y\rangle = \sum\limits^g_{i=1}(x_{2i-1}y_{2i} - x_{2i}y_{2i-1})
\end{array}
$$
with  $\langle x,y \rangle = -\langle y,x\rangle$. If $x\in\bR^{2g}$ has $\langle x,y\rangle =0$ for all $y\in\bR^{2g}$ then $x=0$.

For a suitable basis $v_1,\dots,v_g,w_1,\dots,w_g$ of $\bR^{2g}$, we have
$\langle v_i,v_j \rangle = 0 = \langle w_i,w_j\rangle$, and $\langle v_i,w_j\rangle=1$ 
if $i=j$ and $0$ otherwise. The matrix of the symplectic form with respect
to such a basis is given by
\[ J = \begin{pmatrix} 0 & I \\ -I & 0 \end{pmatrix} \]
where $I$ is the $g\times g$ identity matrix.

The symplectic group $\Sp(2g,\bR)$ consists of the linear 
transformations $\alpha\colon \bR^{2g} \to \bR^{2g}$
which preserve the symplectic form, in the sense that for all $x,y\in\bR^{2g}$ we have
$\langle \alpha(x),\alpha(y) \rangle = \langle x,y\rangle$. This is equivalent to the statement that if $X$ is the matrix for $\alpha$ then $X^tJX=J$.

\begin{eg}\label{eg:symlag}
The lagrangians of $(\bR^{2g},\langle~,~\rangle)$ are the subspaces
$\alpha(\bR^g \oplus 0) \subset \bR^{2g}$  for $\alpha \in \Sp(2g,\bR)$.\\
\hfill\qed
\end{eg}

We shall use the group inclusion
$$S^1 \xymatrix{\ar[r]^-{\displaystyle{\cong}}&} \SO(2)\subset \Sp(2,\bR)~;~
e^{2\pi i a} \mapsto \begin{pmatrix} \cos 2\pi a & -\sin 2\pi a\\
\sin 2\pi a & \cos 2\pi a \end{pmatrix}$$
as an identification.

\begin{eg}\label{eg:mu1}
Let $g=1$. The space ${\mathcal L}_1$ of the lagrangians of the nonsingular symplectic form over $\bR^2$
$$(V,\fa)~=~(\bR\oplus \bR, \begin{pmatrix} 0 & 1 \\ -1 & 0 \end{pmatrix})$$
consists of all the 1-dimensional subspaces $L \subset \bR^2$, which are of the type 
$$L_a~=~\mathsf{Im}\left(\begin{pmatrix} \cos \pi a \\ \sin \pi a \end{pmatrix}:\bR \to \bR \oplus \bR\right) \subset \bR \oplus \bR~(a \in [0,1))~,$$
with an injection
$${\mathcal L}_1 \to \Sp(2,\bR)~;~L_a \mapsto e^{2 \pi i a }=\begin{pmatrix}
\cos 2 \pi a & -\sin 2 \pi a \\
\sin 2 \pi a & \cos 2\pi a
\end{pmatrix}~.$$
For any $a_1,a_2,a_3 \in [0,1)$ the inclusions 
$$j_i~=~\begin{pmatrix} \cos \pi a_i \\ \sin \pi a_i \end{pmatrix}:\bR \to \bR \oplus \bR~(i=1,2,3)$$
with images the lagrangians $j_i(\bR)=L_{a_i} \subset \bR \oplus \bR$ are such that
$$j_i^*\fa j_k~=~\sin \pi(a_k-a_i)~:~\bR \to \bR~.$$
As in Lemma \ref{le:wall} (ii) there is defined an isomorphism of symmetric forms over $\bR$ 
$$\begin{array}{l}
f~:~(\Delta(L_{a_1},L_{a_2},L_{a_3}),\fb)\\[1ex]
=~(\mathsf{ker}(\begin{pmatrix} \cos \pi a_1 & \cos \pi a_2 & \cos\pi a_3 \\
\sin  \pi a_1 & \sin \pi a_2 & \sin \pi a_3 \end{pmatrix}:\bR\oplus \bR \oplus \bR \to \bR\oplus \bR),
\begin{pmatrix} 0 & 1 & 0 \\ 0 & 0 & 0 \\ 0 & 0 & 0 \end{pmatrix})\\[1ex]
\xymatrix{\ar[r]^-{\cong}&} (\Delta'(L_{a_1},L_{a_2},L_{a_3}),\fb')\\[1ex]
=~(\mathsf{ker}(\begin{pmatrix}
\sin \pi(a_1-a_3)& \sin\pi(a_2-a_3) \end{pmatrix}:\bR \oplus \bR\to \bR),
\begin{pmatrix} 0 & \sin \pi(a_2-a_1) \\ 0 & 0 \end{pmatrix})~. 
\end{array}$$
If $a_1,a_2,a_3$ are not all distinct then $\fb=0$, and 
$\mu(L_{a_1},L_{a_2},L_{a_3})=0$.
If $a_2 \neq a_3$ then Lemma \ref{le:wall} (iii) gives an isomorphism
$$\begin{pmatrix}
1 \\ -(j_3^*\fa j_2)^{-1}(j_3^*\fa j_1)\end{pmatrix}~:~
(\bR,-(j_1^*\fa j_2)(j_3^*\fa j_2)^{-1}(j_3^*\fa j_1))
\xymatrix{\ar[r]^-{\cong}&} (\Delta',\fb')~.
$$
It follows that for any $a_1,a_2,a_3 \in [0,1)$ the Wall-Maslov index is
$$\begin{array}{ll}
\mu(L_{a_1},L_{a_2},L_{a_3})&=~
\sigma(\Delta (L_{a_1},L_{a_2},L_{a_3}),\fb)\\[1ex]
&=~\sigma(\Delta' (L_{a_1},L_{a_2},L_{a_3}),\fb')\\[1ex]
&=~\sigma(\bR,-\sin \pi(a_1-a_2) \sin\pi(a_2-a_3) \sin \pi(a_3-a_1))\\[1ex]
&=~-\sign(\sin \pi(a_1-a_2) \sin\pi(a_2-a_3) \sin \pi(a_3-a_1))~.
\end{array}$$
\hfill\qed
\end{eg}

\begin{lemma}\label{le:Maslov-invariant}
If $\alpha\in\Sp(2g,\bR)$ then $\mu(\alpha(L_1),\alpha(L_2),\alpha(L_3))= \mu(L_1,L_2,L_3)$.
\end{lemma}
\begin{proof}
This is clear from the definition.
\end{proof}

\begin{lemma}\label{le:Maslov-cocycle}
If $L_1$, $L_2$, $L_3$, $L_4$ are lagrangians in $\bR^{2g}$ then 
\[ \mu(L_1,L_2,L_3)-\mu(L_1,L_2,L_4)+\mu(L_1,L_3,L_4)-\mu(L_2,L_3,L_4)=0. \]
\end{lemma}
\begin{proof}
See for example Py \cite{Py:2005a}, Th\'eor\`eme (2.2.1).
\end{proof}

Now suppose that $\bR^{2g+2}$ is formed by adjoining new basis elements 
$v_{g+1}$ and $w_{g+1}$. Then given any lagrangian $L$ in $\bR^{2g}$, we may form
the lagrangian $\tilde L$ in $\bR^{2g+2}$ spanned by $L$ and $v_{g+1}$. 

\begin{lemma}\label{le:Maslov-restricts}
Setting $\tilde \Delta = \Delta(\tilde L_1,\tilde L_2,\tilde L_3)$, we have $\tilde \Delta = \Delta \oplus \bR^2$,
and the symmetric form $\fb$ on $\tilde\Delta$ is the direct sum of the form on $\Delta$ 
with the zero form on $\bR^2$. In particular, we have
\[ \mu(\tilde L_1,\tilde L_2,\tilde L_3) = \mu(L_1,L_2,L_3). \]
\end{lemma}
\begin{proof}
The space $\tilde \Delta$ consists of vectors
\[ (a+\lambda v_{g+1},b+\mu v_{g+1},c+ \nu v_{g+1}) \]
with $(a,b,c)\in \Delta$ and $\lambda+\mu+\nu=0$. We have
\begin{align*} 
\fq(a+\lambda v_{g+1},b+\mu v_{g+1},c+\nu v_{g+1}) &= \langle b,a\rangle 
+  \mu \langle v_{g+1},a\rangle + \lambda \langle b,v_{g+1}\rangle + 
\lambda\mu\langle v_{g+1},v_{g+1}\rangle \\
&= \langle b,a\rangle. 
\qedhere
\end{align*}
\end{proof}

\begin{lemma}\label{le:graph} 
Let $(V,\fa)$ be a nonsingular symplectic form over $\bR$.\\
{\rm (i)} The graph of an automorphism $\alpha:(V,\fa) \to (V,\fa)$ is a lagrangian of
$(V \oplus V,\fa \oplus -\fa)$
$$\grph(\alpha)~=~{\rm im}(\begin{pmatrix} 1 \\ \alpha \end{pmatrix}:
V \to V \oplus V) \subset V \oplus V~.$$
{\rm (ii)} For any automorphisms $\alpha_i:(V,\fa) \to (V,\fa)$ $(i=1,2,3)$ let
$$j_i~=~\begin{pmatrix} 1 \\ \alpha_i \end{pmatrix}~:~ (V,0) \to (V \oplus V,\fa \oplus -\fa)$$
be the inclusions of the three graph lagrangians. For $i \neq k$
$$j_i^*(\fa \oplus -\fa)j_k~=~\fa-\alpha_i^* \fa \alpha_k~=~
\fa(1-\alpha_i^{-1}\alpha_k)~:V \to V^*~,$$
so that
$$\begin{array}{l}
(\Delta'(\grph(\alpha_1),\grph(\alpha_2),\grph(\alpha_3)),\fb')\\[1ex]
\hskip50pt
=~(\mathsf{ker}((1-\alpha_3^{-1}\alpha_1~1-\alpha_3^{-1}\alpha_2):V \oplus V \to V),\begin{pmatrix} 0 &\fa(1-\alpha_1^{-1} \alpha_2)\\
0 & 0 \end{pmatrix})~.
\end{array}$$
If one of $1-\alpha_i^{-1} \alpha_k$ is $0$ then $\fb'=0$ and
$\mu(\grph(\alpha_1),\grph(\alpha_2),\grph(\alpha_3))=0$. If $1-\alpha^{-1}_3 \alpha_2:V \to V$ is an isomorphism there is defined
an isomorphism of symmetric forms 
$$\begin{array}{l}
\begin{pmatrix}
1 \\ -(\fa-\alpha_3^*\fa \alpha_2)^{-1}(\fa - \alpha_3^*\fa \alpha_1)\end{pmatrix}~:~
(V,-(\fa-\alpha_1^*\fa \alpha_2)(\fa-\alpha_3^*\fa \alpha_2)^{-1}(\fa-\alpha_3^*\fa \alpha_1))\\[1ex]
\hskip100pt\xymatrix{\ar[r]^-{\cong}&} (\Delta'(\grph(\alpha_1),\grph(\alpha_2),\grph(\alpha_3)),\fb')~,
\end{array}
$$
so that
$$\begin{array}{l}
\mu(\grph(\alpha_1),\grph(\alpha_2),\grph(\alpha_3))\\[1ex]
\hskip50pt=~
\sigma(V,-(\fa-\alpha_1^*\fa \alpha_2)(\fa-\alpha_3^*\fa \alpha_2)^{-1}(\fa-\alpha_3^*\fa \alpha_1))\\[1ex]
\hskip50pt=~\sigma(V,-\fa(1-\alpha_1^{-1}\alpha_2)(1-\alpha_3^{-1} \alpha_2)^{-1}(1-\alpha_3^{-1} \alpha_1))~.
\end{array}
$$
\end{lemma}
\begin{proof} (i) By construction.\\
(ii) Apply Lemma \ref{le:wall}.\\
\end{proof}

\begin{defn}\label{df:Meyercocycle}
The \emph{Meyer cocycle}\index{Meyer cocycle} $\tau_g\colon \Sp(2g,\bR)^\delta \times \Sp(2g,\bR)^\delta \to \bZ$ is defined by
\[ \tau_g(\alpha,\beta) = \mu(\grph(1),\grph(\alpha),\grph(\alpha\beta)). \]
\hfill\qed
\end{defn}

\begin{rk}
It follows from Lemma \ref{le:Maslov-cocycle} that $\tau_g$ is a cocycle on $\Sp(2g,\bR)^\delta$.
By Lemma \ref{le:Maslov-invariant} we have 
\[ \tau_g(\alpha,\beta)=\mu(\grph(\alpha^{-1}),\grph(1),\grph(\beta)). \]
So the subspace $\Delta$ consists of triples
\[ ((x,\alpha^{-1}(x)),(-x-y,-x-y),(y,\beta(y))) \]
with $x,y \in \bR^{2g}$ such that 
$\alpha^{-1}(x)+\beta(y)=x+y$. Thus $\Delta$ is isomorphic to the
space 
\[ \{(x,y)\in\bR^{2g} \oplus \bR^{2g} \mid (\alpha^{-1}-1)x +(\beta-1)y =0\}, \]
with symmetric form
$$\fb((x,y),(x',y'))~=~\langle x+y,(1-\beta)y'\rangle~.$$
This is the definition found in Meyer \cite{Meyer:1973a}, except that the original cocycle was
on $\Sp(2g,\bZ)^{\delta}$.\\
\hfill\qed
\end{rk}

\begin{eg} \label{eg:tau1}
Let $(V,\fa)=(\bR \oplus \bR,\begin{pmatrix}  0 & 1 \\ -1 & 0 \end{pmatrix})$, so that identifying $V=\bC$ have $\fa=-i=e^{-\pi i /2}$. For $a \in [0,1)$ let
$$\begin{array}{l}
\alpha~=~e^{2\pi i a}~=~\begin{pmatrix} \cos 2 \pi a &  -\sin 2 \pi a \\
 \sin 2 \pi a &   \cos 2 \pi a  \end{pmatrix}   \in \Aut(V,\fa)=\Sp(2,\bR)~, \end{array} $$
so that
 $$ 1-\alpha~=~(2 \sin \pi a) e^{\pi i(a +1/2)}~
 =~(2 \sin \pi a) \begin{pmatrix}  \sin \pi a &
 \cos \pi a \\
 -\cos \pi a & \sin \pi a \end{pmatrix}~.$$
 (i) For any $a_1,a_2,a_3 \in [0,1)$ let $\alpha_j=e^{2\pi i a_j}$ $(j=1,2,3)$.
 By Lemma \ref{le:graph} (ii) the Wall-Maslov index of the graph lagrangians
 $\grph(\alpha_j)$ in $(V \oplus V,\fa \oplus -\fa)$ is
  $$\begin{array}{l}
\mu(\grph(\alpha_1),\grph(\alpha_2),\grph(\alpha_3))\\[1ex]
 =~\sigma(V,-\fa(1-\alpha^{-1}_1\alpha_2))(1-\alpha_3^{-1}\alpha_2)^{-1}(1-\alpha_3^{-1}\alpha_1))\\[1ex]
 =~\sigma(V,-e^{-\pi i /2}((2 \sin \pi (a_2-a_1)) e^{\pi i(a_2-a_1 +1/2)}) 
 ((2 \sin \pi (a_2-a_3) ) e^{\pi i(a_2-a_3 +1/2)})^{-1}\\[1ex]
 \hskip150pt ((2 \sin \pi (a_1-a_3)) e^{\pi i(a_1-a_3 +1/2)}))\\[1ex]
 =~ \sigma(V,\dfrac{-2\sin \pi (a_2-a_1) \sin \pi(a_1-a_3)}{\sin \pi (a_2-a_3)})\\[1ex]
 =~-2 \sign( \sin \pi (a_1-a_2) \sin \pi (a_2-a_3) \sin \pi (a_3-a_1)) \in \{0,2,-2\}~.
 \end{array}$$ 
  (ii)  By (i) the evaluation of the Meyer cocycle on  $\alpha=e^{2\pi i a}$, $\beta=e^{2\pi i b} \in \Sp(2,\bR)$ is
 $$\begin{array}{ll}
\tau_1(\alpha,\beta)& =~\mu(\grph(1),\grph(\alpha),\grph(\alpha\beta))\\[1ex]
&=~-2 \sign( \sin \pi a \sin \pi b \sin \pi (a+b)) \in \{0,2,-2\}~.
 \end{array}$$ 
\hfill\qed
\end{eg}

We now consider another cocycle $\tau'_g$ on $\Sp(2g,\bR)^\delta$, again defined 
in terms of the Maslov index. We shall see in Theorem \ref{th:tautau'} below that it is cohomologous to the Meyer cocycle $\tau_g$, but not equal to it. (For $g=1$ see Example \ref{eg:tauprime1}).

\begin{defn}\label{df:Maslovcocycle}
The \emph{Maslov cocycle}\index{Maslov cocycle}
$\tau'_g \colon \Sp(2g,\bR)^\delta \times \Sp(2g,\bR)^\delta \to \bZ$
is defined as follows. Choose a lagrangian subspace $L \subseteq
\bR^{2g}$, and set
\[ \tau'_g(\alpha,\beta) = \mu(L,\alpha(L),\alpha\beta(L)). \]
It follows from Lemma \ref{le:Maslov-invariant} that this is 
independent of the choice of $L$, and that
\[ \tau'_g(\alpha,\beta) = \mu(\alpha^{-1}(L),L,\beta(L)). \]
\hfill\qed
\end{defn}

\begin{eg}\label{eg:tauprime1}
Using the inclusion
$$[0,1) \xymatrix{\ar[r]^-{\cong}&} \SO(2)\subset\Sp(2,\bR)~;~a \mapsto e^{2\pi i a}=
\begin{pmatrix} \cos 2\pi a & -\sin 2\pi a \\
\sin 2\pi a & \cos 2\pi a \end{pmatrix}$$
as an identification we have that for $g=1$ Example \ref{eg:tau1} gives the Meyer cocycle on $[0,1)$ to be
$$\tau_1~:~[0,1) \times [0,1) \to \bZ~;~
(a,b) \mapsto -2\sign(\sin \pi a \sin \pi b \sin \pi (a+b))~.$$
The Maslov cocycle is given by
$$\tau'_1~:~[0,1] \times [0,1] \to \bZ~;~
(a,b) \mapsto \mu(L_0,L_{2\pi a},L_{2\pi (a+b)})=-\sign(\sin 2\pi a \sin 2\pi b \sin (2\pi (a+b)))~.$$
The Dedekind $((~))$-function is defined by
$$((~))~:~\bR \to (-1/2,1/2) ~;~ x \mapsto ((x))~=~
\begin{cases} \{x\}-1/2&{\rm if}~x \in \bR\backslash \bZ\\
0&{\rm if}~x \in \bZ \end{cases}$$
with $\{x\} \in [0,1)$ the fractional part of $x \in \bR$, and is such that
$$\begin{array}{l}
2((2x))-4((x))~=~\sign(\sin 2\pi x)~,\\[1ex]
2(\,((x))+((y))-((x+y))\,)~=~-\sign(\sin \pi x \sin \pi y \sin \pi(x+y))~.
\end{array}$$
Thus
$$\begin{array}{l}
\tau_1(a,b)~=~-4(\,((a))+((b))-((a+b))\,)~,\\[1ex]
\tau'_1(a,b)~=~-2(\,((2a))+((2b))-((2a+2b))\,)~,\\[1ex]
\tau_1(a,b)-\tau'_1(a,b)~=~-\sign(\,\sin 2\pi a)-\sign(\sin 2\pi b)+\sign(\sin 2\pi(a+b)) \in \bZ
\end{array}
$$
and 
$$[\tau_1]~=~[\tau'_1] \in H^2(\Sp(2,\bR)^\delta,\bZ)~.$$
\hfill\qed
\end{eg}

\begin{prop}\label{pr:cocycles-restrict}
Embed $\bR^{2g}$ in $\bR^{2g+2}$ by adjoining new basis elements
$v_{g+1}$ and $w_{g+1}$, and consider the corresponding embedding
$\Sp(2g,\bR)^\delta \to \Sp(2g+2,\bR)^\delta$. 
\begin{enumerate}
\item[\rm (i)] The Maslov cocycle $\tau'_{g+1}$ on $\Sp(2g+2,\bR)^\delta$ restricts to
the Maslov cocycle $\tau'_g$ on $\Sp(2g,\bR)^\delta$.
\item[\rm (ii)] The Meyer cocycle $\tau_{g+1}$ on $\Sp(2g+2,\bR)^\delta$ restricts to
the Meyer cocycle $\tau_g$ on $\Sp(2g,\bR)^\delta$.
\end{enumerate}
\end{prop}
\begin{proof}
(i) This follows immediately from Lemma \ref{le:Maslov-restricts}.

(ii) For $\alpha\in\Sp(2g,\bR)^\delta$, the graph of $\alpha$ considered as 
an element of $\Sp(2g+2,\bR)^\delta$ is the direct sum of the graph of $\alpha$
considered as an element of $\Sp(2g,\bR)^\delta$ and $\grph(1)\subset
\bR^2\oplus \bR^2$. So apply Lemma \ref{le:Maslov-restricts} twice.
\end{proof}
